# Supplementary material for: NARRATE: Versatile Language Architecture for Optimal Control in Robotics
Source: arXiv:2403.10762 source file (2024-03-16)
Supplement: Supplementary file 2 [file appendixB.tex]

\subsection{Dynamics and Control of the Franka Robotic Arm} \label{appendix:dynamics}

\subsubsection{Linearized Model} \label{apendix:linear_model}
The linear dynamics used in this work are as follows
\begin{equation*}
\begin{aligned}
    \begin{bmatrix}
    x_{t+1} \\
    y_{t+1} \\
    z_{t+1} \\
    \Dot{x}_{t+1} \\
    \Dot{y}_{t+1} \\
    \Dot{z}_{t+1}
    \end{bmatrix} =&
    \begin{bmatrix}
    1 & 0 & 0 & \Delta \tau & 0 & 0 \\
    0 & 1 & 0 & 0 & \Delta \tau & 0 \\
    0 & 0 & 1 & 0 & 0 & \Delta \tau \\
    0 & 0 & 0 & 0 & 0 & 0 \\
    0 & 0 & 0 & 0 & 0 & 0 \\
    0 & 0 & 0 & 0 & 0 & 0 \\
    \end{bmatrix}
    \begin{bmatrix}
    x_t \\
    y_t \\
    z_t \\
    \Dot{x}_t \\
    \Dot{y}_t \\
    \Dot{z}_t 
    \end{bmatrix}
    + \\
    & \hspace{3.5cm}
    +\begin{bmatrix}
    0 & 0 & 0 \\
    0 & 0 & 0 \\
    0 & 0 & 0 \\
    1 & 0 & 0 \\
    0 & 1 & 0 \\
    0 & 0 & 1 \\
    \end{bmatrix}
    \begin{bmatrix}
    u_{x,t} \\
    u_{y,t} \\
    u_{z,t} \\
    \end{bmatrix},
    \label{eq: pm_model}
\end{aligned}
\end{equation*}
where the state $ [x, y ,z, \Dot{x}, \Dot{y}, \Dot{z}]^T$ represents the 3D position and velocity of the robot gripper. The control actions are $\textbf{u} = [u_x, u_y, u_z]^T$, and virtually represent the gripper velocity. $\Delta \tau = 0.1$ represents the dicretization time since the model is provided already in discrete form. 

Notice that the system cannot be readily controllable with this model since it does not capture in any way the underlying physics of the robot manipulator, hence the need for the TT block. Moreover, do not even have direct access to the gripper velocity. Nevertheless the output simply acts as a reference that the TT will try to match as closely as possible.

\subsubsection{MPC versus Reinforcement Learning for the TG block} \label{appendix:RL_vs_MPC}

Although MPC is the controller of choice in this formulation, we note that Reinforcement Learning (RL) policies can be similarly implemented since both schemes are solving the Optimal Control Problem (OCP) \cite{Pontryagin2018} \cite{Berkovitz1974}. 
Given a system with states $\textbf{x}$, in order to compute actions $\textbf{u}$, the OCP is formulated as an optimazation problem over an (infinite) horizon:
\begin{subequations}\label{eq: OCP}
\begin{align}
\underset{\pi_t}{\text{min}} & \qquad \sum_{t=0}^{\bar{T}} \gamma^t r(x_t, u_t) \label{eq:ocp_cost}  \\
 & \qquad x_{t+1} = S(x_t, u_t, w_t; \theta) \label{eq:ocp_dyanimcs} \\
 & \qquad u_t = \pi_t(x_0,...,x_t,u_0,...,u_{t-1}) \label{eq:ocp_policy} \\
 & \qquad x_k \in\mathcal{X}_t, \quad u_t \in\mathcal{U}_t  \label{eq:ocp_state_set} \\
 & \qquad x_0 =  x_{init}, \qquad \forall t=0,\dots,\bar{T}\label{eq:ocp_init},
\end{align}
\end{subequations}
where $x$ and $u$ represent the state and action respectively, and $T$ indicates the full horizon length and is not constrained to be finite.

In this formulation, equation (\ref{eq:ocp_cost}) represents the OCP cost (or reward) function that needs to be minimized (or maximized) and it depends on the state and action sequences $x,\ u$. Equation (\ref{eq:ocp_dyanimcs}) represents the dynamics function and computes the state at the next time step $x(t+1)$ as function of the current state $x(t)$, control action $u(t)$ and disturbance $w(t)$ while being parametrized  by $\theta$. Equation (\ref{eq:ocp_policy}) shows that the control action $u(t)$ is computed by a policy function $\pi_t$ which takes as input the previous states and controls. Constraint (\ref{eq:ocp_state_set}) impose the states and actions to be within their corresponding feasible set. Finally Equation (\ref{eq:ocp_init}) imposes that the state at the zeroth time step $\textbf{x}(0)$ in the optimization problem is initialized to the current measurement of the state of the system. \\

The OCP as formulated in Equations (\ref{eq:ocp_cost}) - (\ref{eq:ocp_init}) is often intractable and assumptions or simplifications need to be made in order to be solved. Here is where the main difference lies between and MPC and an RL-based controller.

On one hand, the simplifications made by RL are:
\begin{itemize}
    \item The cost function is evaluated empirically by fitting a value function $V^{\pi_t}(x(t))$ to the rewards received for each state at each episode under policy $\pi_t$. 
    \item The problem is solved in iterative improvements by learning the policy during rollout. This approach is generally model free, meaning that Equation (\ref{eq:ocp_dyanimcs}) is omitted and the policy function $\pi$ learns to map state to action directly throughout episodic learning. Due to the nature of learning across multiple episodes, constraints in Equations (\ref{eq:ocp_state_set}) - (\ref{eq:ocp_action_set}) cannot be applied and have to be omitted. Although constraint violation can be penalized in the value function $V^{\pi}(\cdot)$ by adding regularization terms that need to be hand designed, there are no guarantees that the learned policy will satisfy the original constraints. 
\end{itemize}

On the other hand, the main assumptions made by MPC are:
\begin{itemize}
    \item While Equations (\ref{eq:ocp_cost}) - (\ref{eq:ocp_init}) are kept in the formulation, they are generally simplified in order to be solved via numerical optimization. This means that cost, dynamics and constraint functions are approximated when needed. For example disturbances $w(t)$ may be omitted from the formulation, and  dynamics parameters $\theta$ may be assumed to be fixed. While imposing the presence of dynamics and constraints, MPC does not require them to be known a priori but they can actually be learnt in a data-driven approach while the controller is operating \cite{}, similar to RL-based policies.
    \item The problem is solved via numerical optimization in a receding horizon fashion. The original horizon $\bar{T}$ is reduced to a shorter horizon $T$. The problem is then solved for the reduced horizon and only the first control action $u_0$ is applied. The states are then newly measured and the MPC problem is solved again with the new measurement of the state as $x_{init}$. To account for the shorter horizon, a terminal cost function is generally added to better approximate the OCP problem, this function can be designed or, similarly to RL, a value function can be learnt iteratively.
\end{itemize}

\subsubsection{PD Controller} \label{apendix:PD_controller}

The dynamics model of a robot manipulator can be generally described as
\begin{equation*}
    M(q) \Ddot{q} + b(q), \Dot{q}) + g(q) = \tau + J_c^T(q) F_c,
    \label{eq: eom}
\end{equation*}
where $q$, $\Dot{q}$, and $\Ddot{q}$ are the generalized position, velocity and acceleration vectors of robot joints, $M(q)$ is the generalized mass matrix (orthogonal), $b(q, \Dot{q})$ represents the Coriolis and centrifugal terms, 
$g(q)$ accounts for the gravitational terms,
$J_c(q)$ is the geometric Jacobian corresponding to the external forces, and $F_c$ are the external Cartesian forces (e.g. from contacts). $\tau$ represents the motor torques that need to be applied to the robot motors in order to follow the trajectory received from the trajectory planner. 

Once $w$ is computed according to the PD gains as per equation \eqref{eqn:PD_controller}, the desired motor torques can then be computed as:
\begin{equation}
    \tau = J_e^T (\Lambda \Dot{w}^* + \mu + r),
\end{equation}
where $J_e$, $\Lambda$, $\mu$, and $r$ are obtained from the dynamics model.
