# Supplementary material for: NARRATE: Versatile Language Architecture for Optimal Control in Robotics
Source: arXiv:2403.10762 source file (2024-03-16)
Supplement: Supplementary file 3 [file appendixC.tex]

\subsection{Experiments} \label{appendix:experiments}

\subsubsection{Stack}
\paragraph{Plan}
Given the task of stacking all cubes on top of each other, the TP generates the following successful plan:
\begin{tcolorbox}[
    colframe=darkgray, % Dark grey frame color
    boxrule=0.2pt, % Frame thickness
    colback=lightgray!20, %
    arc=3pt, % Rounded corners
    fontupper=\small,
    breakable,
    halign=left
    ]
    
Plan(tasks=[ \\
\quad "move the gripper to cube\_4 and avoid any collision with every cube", \\
\quad  "close gripper", \\
\quad  "move the gripper above cube\_2 and avoid colliding with cube\_2, cube\_3 and cube\_1", \\
\quad  "open gripper", \\
\quad  "move gripper to cube\_3 and avoid collisions with every cube", \\
\quad  "close gripper", \\
\quad  "move gripper above of cube\_4 and avoid collisions with every cube apart from cube\_3", \\
\quad  "open gripper", \\
\quad  "move gripper to cube\_1 and avoid collisions with every cube", \\
\quad  "close gripper", \\
\quad  "move gripper above cube\_3 and avoid collisions with every cube apart from cube\_1", \\
\quad  "open gripper" \\
])

\end{tcolorbox}

\paragraph{Optimization}
Given the task to go to a cube\_1 and avoid collisions with all cubes, the following optimization is applied:
\begin{tcolorbox}[
    colframe=darkgray, % Dark grey frame color
    boxrule=0.2pt, % Frame thickness
    colback=lightgray!20, %
    arc=3pt, % Rounded corners
    fontupper=\small,
    breakable,
    halign=left
    ]

    Optimization(\\
        \qquad objective= "ca.norm\_2(x - cube\_1 + )**2", \\
        \qquad equality\_constraints = [],\\
        \qquad inequality\_constraints= [ \\
        \quad \qquad  "d\_min - ca.norm\_2(x - cube\_1)", \\
        \quad \qquad  "d\_min - ca.norm\_2(x - cube\_2)", \\
        \quad \qquad  "d\_min - ca.norm\_2(x - cube\_3)", \\
        \quad \qquad  "d\_min - ca.norm\_2(x - cube\_4)" \\
        \qquad ]\\
    )

\end{tcolorbox}

Given the task to go above cube\_2, the following optimization is successfully applied:
\begin{tcolorbox}[
    colframe=darkgray, % Dark grey frame color
    boxrule=0.2pt, % Frame thickness
    colback=lightgray!20, %
    arc=3pt, % Rounded corners
    fontupper=\small,
    breakable,
    halign=left
    ]

    Optimization(\\
        \qquad objective= "ca.norm\_2(x - cube\_2 + np.array([0, 0, 0.468]))**2", \\
        \qquad equality\_constraints = [],\\
        \qquad inequality\_constraints= [ \\
        \quad \qquad  "d\_min - ca.norm\_2(x - cube\_2)", \\
        \quad \qquad  "d\_min - ca.norm\_2(x - cube\_3)", \\
        \quad \qquad  "d\_min - ca.norm\_2(x - cube\_4)" \\
        \qquad ]\\
    )

\end{tcolorbox}

\subsubsection{Pyramid}

\paragraph{Plan}
Given the task of building a pyramid, the TP generates the following successful plan:

\begin{tcolorbox}[
    colframe=darkgray, % Dark grey frame color
    boxrule=0.2pt, % Frame thickness
    colback=lightgray!20, %
    arc=3pt, % Rounded corners
    fontupper=\small,
    breakable,
    halign=left
    ]

Plan(tasks=[ \\
\quad  "move the gripper to cube\_4 and avoid any collision with every cube", \\
\quad  "close gripper", \\
\quad  "move the gripper next to cube\_3 and avoid colliding with cube\_2, cube\_3 and cube\_1", \\
\quad  "open gripper", \\
\quad  "move gripper to cube\_2 and avoid collisions with every cube", \\
\quad  "close gripper", \\
\quad  "move gripper at a height above cube\_3 and cube\_4 and in between them. Also avoid collisions with every cube apart from cube\_2", \\
\quad  "open gripper" \\
])
\end{tcolorbox}
\subsubsection{Optimization}
Similar to \textit{Stack}.

\subsubsection{L}
\paragraph{Plan}
Given the task of rearranging the cubes to form the letter L, the TP generates the following successful plan:

\begin{tcolorbox}[
    colframe=darkgray, % Dark grey frame color
    boxrule=0.2pt, % Frame thickness
    colback=lightgray!20, %
    arc=3pt, % Rounded corners
    fontupper=\small,
    breakable,
    halign=left
    ]

Plan(tasks=[ \\
\quad  "move the gripper to cube\_4 and avoid any collision with every cube", \\ 
\quad  "close gripper", \\
\quad  "move the gripper in front cube\_2 and avoid colliding with cube\_2, cube\_3 and cube\_1", \\ 
\quad  "open gripper", \\ 
\quad  "move gripper to cube\_3 and avoid collisions with every cube", \\ 
\quad  "close gripper", \\
\quad  "move gripper in behind cube\_2 and avoid collisions with cube\_1, cube\_2, cube\_4", \\
\quad  "open gripper", \\
\quad  "move gripper to cube\_1 and avoid collisions with every cube", \\ 
\quad  "close gripper", \\
\quad  "move gripper to the right of cube\_3 and avoid colliding with cube\_3", \\ 
\quad  "open gripper", \\
])

\end{tcolorbox}
\paragraph{Optimization}
Similar to \textit{Stack}.

\subsubsection{Clean Plate}
\paragraph{Plan}
Given the task of cleaning a plate with a sponge, the TP generates the following successful plan:

\begin{tcolorbox}[
    colframe=darkgray, % Dark grey frame color
    boxrule=0.2pt, % Frame thickness
    colback=lightgray!20, %
    arc=3pt, % Rounded corners
    fontupper=\small,
    breakable,
    halign=left
    ]

Plan(tasks:[\\
  \quad "move the gripper to the sponge", \\
  \quad "close gripper", \\
  \quad "move the gripper upwards 0.05m", \\
  \quad "move the gripper 0.02m above the plate avoiding collision with the plate", \\
  \quad "move the gripper in circular motion over the plate with radius equal to the plate's radius"\\
])

\end{tcolorbox}
\paragraph{Optimization}
The task of picking and moving the sponge is similar to \textit{Stack} for the cubes. The task of moving the gripper in a circular motion over the plate is converted into the following:
\begin{tcolorbox}[
    colframe=darkgray, % Dark grey frame color
    boxrule=0.2pt, % Frame thickness
    colback=lightgray!20, %
    arc=3pt, % Rounded corners
    fontupper=\small,
    breakable,
    halign=left
    ]

    Optimization(\\
        \qquad objective= "ca.norm\_2(x - plate + np.array([radius*np.cos(t), radius*np.sin(t), 0]))**2", \\
        \qquad equality\_constraints = [],\\
        \qquad inequality\_constraints= []\\
    )

\end{tcolorbox}

\subsubsection{Move Sponge}
\paragraph{Plan}
Given the task of moving the sponge to the sink, the TP generates the following successful plan:

\begin{tcolorbox}[
    colframe=darkgray, % Dark grey frame color
    boxrule=0.2pt, % Frame thickness
    colback=lightgray!20, %
    arc=3pt, % Rounded corners
    fontupper=\small,
    breakable,
    halign=left
    ]

Plan(tasks:[\\
  \quad "Left robot: move gripper above the sponge and avoid colliding with the sponge. Right robot: move gripper above the container handle.", \\ 
  \quad "Left robot: move gripper to the sponge. Right robot: move gripper to the container handle.", \\
  \quad "Left robot: close gripper. Right robot: close gripper", \\
  \quad "Left robot: move the gripper 0.1m above the container. Right robot: nothing", \\
  \quad "Left robot: move the gripper to the sink while staying 0.1m above the container. Right robot: move the gripper to the sink", \\ 
  \quad "Left robot: open gripper to drop the sponge in the sink. Right robot: maintain position under the sponge."\\
])

\end{tcolorbox}
\paragraph{Optimization}
The task of going to the sponge and the container is formulated successfully as:
\begin{tcolorbox}[
    colframe=darkgray, % Dark grey frame color
    boxrule=0.2pt, % Frame thickness
    colback=lightgray!20, %
    arc=3pt, % Rounded corners
    fontupper=\small,
    breakable,
    halign=left
    ]

    Optimization(\\
        \qquad objective= "ca.norm\_2(x_left - sponge + )**2 + ca.norm\_2(x_right - container\_handle)**2", \\
        \qquad equality\_constraints = [],\\
        \qquad inequality\_constraints= []\\
    )

\end{tcolorbox}

The task of enforcing that the container is always under the sponge while moving it to the sink is formulated as follows:
\begin{tcolorbox}[
    colframe=darkgray, % Dark grey frame color
    boxrule=0.2pt, % Frame thickness
    colback=lightgray!20, %
    arc=3pt, % Rounded corners
    fontupper=\small,
    breakable,
    halign=left
    ]

    Optimization(\\
        \qquad objective= "ca.norm\_2(x\_left - sink )**2 + ca.norm\_2(x\_right - sink)**2", \\
        \qquad equality\_constraints = [0 - ca.norm\_2(x\_left[:1] - container[:1])],\\
        \qquad inequality\_constraints= [0.1 - ca.norm\_2(x\_left[2] - container[2]) ]\\
    )

\end{tcolorbox}

\subsubsection{Move table}
\paragraph{Plan}
Given the task of moving a table, the TP generates the following successful plan:

\begin{tcolorbox}[
    colframe=darkgray, % Dark grey frame color
    boxrule=0.2pt, % Frame thickness
    colback=lightgray!20, %
    arc=3pt, % Rounded corners
    fontupper=\small,
    breakable,
    halign=left
    ]

Plan(tasks:[\\
  \quad "Move the left gripper to the left handle and move the right gripper to the right handle", \\
  \quad "Keep the grippers at the handle and make sure to maintain the same distance between the grippers", \\
  \quad "You now can close the grippers",
  "move the grippers 0.15m upwards while keeping the same distance between the grippers", \\
  \quad "Move the grippers 0.5m backwards while making sure the grippers keep the same distance to each other", \\
  \quad "Move the grippers 0.15m downwards while keeping the same distance between the grippers", \\
  \quad "You can now open the grippers" \\
])

\end{tcolorbox}
\paragraph{Optimization}
After both grippers grabbed the table handles, the task of moving the table behind the obstacle while avoiding collisions and enforcing the grippers to remain at the same distace is successfully formulated as:
\begin{tcolorbox}[
    colframe=darkgray, % Dark grey frame color
    boxrule=0.2pt, % Frame thickness
    colback=lightgray!20, %
    arc=3pt, % Rounded corners
    fontupper=\small,
    breakable,
    halign=left
    ]

    Optimization(\\
        \qquad objective= "ca.norm\_2(x\_left - obstacle - np.array([0, 0.35, 0]))**2 + ca.norm\_2(x\_right - obstacle - np.array([0, 0.35, 0]))**2", \\
        \qquad equality\_constraints = [0 - ca.norm\_2(x\_left - x\_right)],\\
        \qquad inequality\_constraints= [radius\_obstacle - table\_height - ca.norm\_2((x\_left + x\_right)) ]\\
    )

\end{tcolorbox}
