# Supplementary material for: NARRATE: Versatile Language Architecture for Optimal Control in Robotics
Source: arXiv:2403.10762 source file (2024-03-16)
Supplement: Supplementary file 4 [file appendixD.tex]

\subsection{Other architectures in the literature} \label{appendix:dynamics}
Here we compare our proposed architecture with other architecture taxonomies as discussed in Section \ref{sec:taxonomy}.

\paragraph{Language-to-action.} The approach in \cite{todo} splits $K$ into two different blocks: $M$ and $N$. Here, $M: \Sigma*\rightarrow \mathbb R^{N_x}$ is computed via a language model, which is used to turn natural language into trajectory points. $N:\mathbb R^{N_x}\rightarrow \mathbb R^{N_u}$ is implemented in a controller, which solves inverse kinematics to retrieve the control inputs that would lead to the trajectory generated by $L$. Since this approach is mostly end-to-end, it is not possible to guarantee constraint satisfaction of the resulting trajectory, and they rely on \emph{a posteriori} sanity check to verify the feasibility of the proposed trajectory.\looseness=-1

\paragraph{Language-to-code.} The approach in \cite{todo} splits $K$ into two different blocks: $P$ and $Q$. Here, $P:\Sigma^*\rightarrow \Sigma^*$ is computed via a language model, which translates natural language strings into Python code. $Q:\Sigma^*\rightarrow R^{N_u}$ is the module executing the code and sending commands to the robot. Given the lack of imposed structure in the generated code, and the lack of reliability of language models, it is impossible to guarantee the feasibility and safety of the resulting trajectory.

\paragraph{Language-to-reward.} The approach in \cite{todo} splits $K$ into three different blocks: $R$, $T$, $V$. Here, $R:\Sigma^*\rightarrow \Sigma^*$ is equivalent to our TG block. $T: \Sigma^*\rightarrow \mathcal {C}\subset C^1$ translates the different subtasks as expressed in natural language into a reward function. Notice that the set of reward functions available to the model is restricted to a set of predefined functions implemented in MJPC \cite{todo}. Lastly, $V$ is equivalent to our control module, where $V: \mathcal {C}\subset C^1 \rightarrow \mathbb R^{N_u}$. We note that since no constraints are explicitly introduced, the trajectories generated have no safety guarantees, such as guarantees for collision avoidance. In \cite{todo}, a promising approach is proposed, where the language model is trained via reinforcement learning to choose appropriate reward functions. However, the lack of guaranteed, such as the ones imposed via hard constraints, is still an issue.
